# Supplementary material for: Properly learning monotone functions via local reconstruction
Source: arXiv:2204.11894 source file (2023-03-27)
Supplement: Supplementary file 1 [file appendixA.tex]

\section*{Appendix A}
Here is a table of LCAs for maximal independent set (copied from a summary in \cite{ghaffari_sparsifying_2018}):

 \begin{tabular}{||c c c ||} 
 \hline
 Paper & Claimed query or time complexity & Seems good enough for us? \\ [0.5ex] 
 \hline\hline
 \cite{AlonRVX12} & $2^{O(\Delta \log^2\Delta )}\log N$  & No\\ 
 \hline
 \cite{reingold_new_2014} &  $2^{O(\Delta)}\log N \log\log N$ & No\\
 \hline
 \cite{even_best_2014} & $2^{O(\Delta^2 \log^2\Delta)}\log^*N$  & No\\
 \hline
 \cite{levi_local_2015} & $2^{O(\log^3\Delta)}\log^3 N$  & Yes\\
 \hline

 \cite{ghaffari_improved_2015} & $2^{O(\log^2\Delta)}\log^3 N$ & Yes \\
  \hline
 \cite{ghaffari_sparsifying_2018} & $2^{O(\log\Delta \log\log\Delta)}\polylog N$ & Yes \\
 [1ex] 
 \hline
\end{tabular}

To really make sure Theorem \ref{theorem: LCA for maximal independent set} is implied by one of the above,
it makes sense to go through one of these papers and see if there is no subtle way in which Theorem \ref{theorem: LCA for maximal independent set} fails to follow.

%(removed, because not directly relevant) First, we observe that if the success probability is $1-\frac{1}{N^C_0}$ for some fixed positive constant $C_0$, then it can be boosted to $1-\frac{1}{N^C}$ for any positive $C$ by adding $\left(\frac{N^C}{N^{C_0}}-1\right)N$ isolated vertices to the graph. Adjacency list access to this new graph can be simulated with constant overhead. If the original run-time, sample complexity and common randomness were as in Theorem \ref{theorem: LCA for maximal independent set}, then after adding these isolated vertices, only the constants in the $O(\cdot)$ terms will get worse.

Now, regretfully  \cite{ghaffari_sparsifying_2018} does not seem to mention anything explicitly about run-time, and it seems complicated to go through everything and make sure the algorithm runs fast enough. 

So I ended up looking at  \cite{ghaffari_improved_2015}. This paper (\cite{ghaffari_improved_2015}) on page 4 explicitly says they have an LCA with time and space complexity $2^{O(\log^2\Delta)}\log^3 N$ and $2^{O(\log^2\Delta)}\log^2 N$ respectively. 

I decided to go through \cite{ghaffari_improved_2015} anyway and make sure I am happy with it, because it only lists the details of a certain distributed algorithm and seems to imply that LCA would be spelled out explicitly in a final version, which seems not to exist. However, a good LCA indeed follows very directly from their main lemma\footnote{After examining the paper, I am confident about $2^{\polylog (\Delta)}\,\polylog (N)$ run-time, sample complexity and common randomness. I think the claimed exponents in the polylogarithmic terms follow too, but I did not bother to check this one too carefully, as we do not really need these specific exponents.}, as I will elaborate. \href{https://www.dropbox.com/s/y6rsh24sc1vbe3l/Ghaffari\%20-\%202015\%20-\%20An\%20Improved\%20Distributed\%20Algorithm\%20for\%20Maximal\%20Inde.pdf?dl=1}{Here} you can find an annotated version in which I crossed over parts I think are not directly relevent to the LCA question and marked main steps and logical implications.

First, the paper defines the following distributed algorithm for MIS (I will refer to it as the desire-level algorithm). Each vertex $v$ at each round $t$ has a "desire-level" $p_t(v)$. This desire level evolves as 
\[
p_{t+1}(v)
=\begin{cases}
p_t(v)/2, &\text{if $\sum_{u\in\{\text{neighbors of $v$}\}}p_t(u)\geq 2$},\\
\min(2p_t(v),1/2) &\text{otherwise}.
\end{cases}
\]
Additionally, at each step $t$ a vertex $v$ gets \textbf{marked} with probability $p_t(v)$. If $v$ gets marked, and no neighbour of $v$ gets marked, then $v$ gets added to MIS, and is removed from the graph together with all its neighbors.

It is clear that by inspecting the $O(\tau)$-neighborhood of a vertex $v$, one can simulate $\tau$ iterations of the algorithm and see if $v$ is still undecided by that time or not. This $O(\tau)$-neighborhood has $\Delta^{O(\tau)}$ member vertices. If the vertex is thus undesided by iteration $\tau$ we call $v$ \textbf{$\tau$-undecided}, and otherwise we call $v$ \textbf{$\tau$-decided}.

The LCA does the following for a vertex $v$:
\begin{itemize}
    \item Take $\tau=\Theta(C\log \Delta)$ with the appropriate constant (recall, $1-1/N^C$ is the desired success probability).
    \item Determine If $v$ is $\tau$-decided. If so, output whether $v$ was included in MIS or not and exit. Otherwise, continue.
    \item For each neighbor of $v$, determine if it is \textbf{$\tau$-decided}. For each \textbf{$\tau$-undecided} neighbor recursively determine which its neighbors in turn are \textbf{$\tau$-undecided}. Continuing this way, find the connected component of \textbf{$\tau$-undecided} vertices around $v$. 
    \item Use a greedy algorithm to make decision which members of this connected component should join the MIS (for example, sort them by their ID-s and greedily add them one-by-one to MIS when possible).
    \item Output whether this greedy procedure decided to add $v$ to MIS.
\end{itemize}
Theorem 4.2 in \cite{ghaffari_improved_2015} says that with probability at least $1-1/N^C$ for every vertex $v$ the connect component of undecided vertices around $v$ will have size at most $O(\log_\Delta N \cdot \Delta^4)$. Determining if a vertex is $\tau$-decided takes $\Delta^{O(\tau)}=2^{O(\log^2\Delta)}$ queries. So, for a vertex $v$ one thus needs $2^{O(\log^2\Delta)}\log N$ queries.

Common randomness can be reduced standardly by using $2^{O(\log^2\Delta)}\log N$-wise independent random variables for deciding if a vertex gets marked or not. We see we can do with $2^{\polylog (\Delta)}\,\polylog (N)$ common randomness.

Going through the algorithm we see that the run-time is also $2^{\polylog (\Delta)}\,\polylog (N)$. Though the exact constants in the polylogarithmic terms do not concern us too much, I suppose if one goes through everything carefully one indeed gets a run-time of $2^{O(\log^2\Delta)}\log^3 N$ as promised.
